# Supplementary material for: Time Advances and Dispersive Constraints in Dressed Gravitational Scattering
Source: arXiv:2611.14721 source file (2026-11-10)
Supplement: Supplementary file 1 [file supplement_references.tex]

%
%
%
%
%
%
%
%
\begin{thebibliography}{9}%
\makeatletter
\providecommand \@ifxundefined [1]{%
 \@ifx{#1\undefined}
}%
\providecommand \@ifnum [1]{%
 \ifnum #1\expandafter \@firstoftwo
 \else \expandafter \@secondoftwo
 \fi
}%
\providecommand \@ifx [1]{%
 \ifx #1\expandafter \@firstoftwo
 \else \expandafter \@secondoftwo
 \fi
}%
\providecommand \natexlab [1]{#1}%
\providecommand \enquote  [1]{``#1''}%
\providecommand \bibnamefont  [1]{#1}%
\providecommand \bibfnamefont [1]{#1}%
\providecommand \citenamefont [1]{#1}%
\providecommand \href@noop [0]{\@secondoftwo}%
\providecommand \href [0]{\begingroup \@sanitize@url \@href}%
\providecommand \@href[1]{\@@startlink{#1}\@@href}%
\providecommand \@@href[1]{\endgroup#1\@@endlink}%
\providecommand \@sanitize@url [0]{\catcode `\\12\catcode `\$12\catcode
  `\&12\catcode `\#12\catcode `\^12\catcode `\_12\catcode `\%12\relax}%
\providecommand \@@startlink[1]{}%
\providecommand \@@endlink[0]{}%
\providecommand \url  [0]{\begingroup\@sanitize@url \@url }%
\providecommand \@url [1]{\endgroup\@href {#1}{\urlprefix }}%
\providecommand \urlprefix  [0]{URL }%
\providecommand \Eprint [0]{\href }%
\providecommand \doibase [0]{https://doi.org/}%
\providecommand \selectlanguage [0]{\@gobble}%
\providecommand \bibinfo  [0]{\@secondoftwo}%
\providecommand \bibfield  [0]{\@secondoftwo}%
\providecommand \translation [1]{[#1]}%
\providecommand \BibitemOpen [0]{}%
\providecommand \bibitemStop [0]{}%
\providecommand \bibitemNoStop [0]{.\EOS\space}%
\providecommand \EOS [0]{\spacefactor3000\relax}%
\providecommand \BibitemShut  [1]{\csname bibitem#1\endcsname}%
\let\auto@bib@innerbib\@empty
%
\bibitem [{\citenamefont {Arkani-Hamed}\ \emph {et~al.}(2021)\citenamefont
  {Arkani-Hamed}, \citenamefont {Pate}, \citenamefont {Raclariu},\ and\
  \citenamefont {Strominger}}]{sm-Arkani-Hamed:2020gyp}%
  \BibitemOpen
  \bibfield  {author} {\bibinfo {author} {\bibfnamefont {N.}~\bibnamefont
  {Arkani-Hamed}}, \bibinfo {author} {\bibfnamefont {M.}~\bibnamefont {Pate}},
  \bibinfo {author} {\bibfnamefont {A.-M.}\ \bibnamefont {Raclariu}},\ and\
  \bibinfo {author} {\bibfnamefont {A.}~\bibnamefont {Strominger}},\ }\bibfield
   {title} {\bibinfo {title} {{Celestial amplitudes from UV to IR}},\ }\href
  {https://doi.org/10.1007/JHEP08(2021)062} {\bibfield  {journal} {\bibinfo
  {journal} {JHEP}\ }\textbf {\bibinfo {volume} {08}}\bibfield  {number}
  {\bibinfo  {number} { (2021)},\ \bibinfo {pages} {062}},\ }\Eprint
  {https://arxiv.org/abs/2012.04208} {arXiv:2012.04208 [hep-th]} \BibitemShut
  {NoStop}%
\bibitem [{\citenamefont {Ware}\ \emph {et~al.}(2013)\citenamefont {Ware},
  \citenamefont {Saotome},\ and\ \citenamefont {Akhoury}}]{sm-Ware:2013zja}%
  \BibitemOpen
  \bibfield  {author} {\bibinfo {author} {\bibfnamefont {J.}~\bibnamefont
  {Ware}}, \bibinfo {author} {\bibfnamefont {R.}~\bibnamefont {Saotome}},\ and\
  \bibinfo {author} {\bibfnamefont {R.}~\bibnamefont {Akhoury}},\ }\bibfield
  {title} {\bibinfo {title} {{Construction of an asymptotic S matrix for
  perturbative quantum gravity}},\ }\href
  {https://doi.org/10.1007/JHEP10(2013)159} {\bibfield  {journal} {\bibinfo
  {journal} {JHEP}\ }\textbf {\bibinfo {volume} {10}}\bibfield  {number}
  {\bibinfo  {number} { (2013)},\ \bibinfo {pages} {159}},\ }\Eprint
  {https://arxiv.org/abs/1308.6285} {arXiv:1308.6285 [hep-th]} \BibitemShut
  {NoStop}%
\bibitem [{\citenamefont {Hannesdottir}\ and\ \citenamefont
  {Schwartz}(2020)}]{sm-HannesdottirSchwartz:2020}%
  \BibitemOpen
  \bibfield  {author} {\bibinfo {author} {\bibfnamefont {H.}~\bibnamefont
  {Hannesdottir}}\ and\ \bibinfo {author} {\bibfnamefont {M.~D.}\ \bibnamefont
  {Schwartz}},\ }\bibfield  {title} {\bibinfo {title} {{$S$ -Matrix for
  massless particles}},\ }\href {https://doi.org/10.1103/PhysRevD.101.105001}
  {\bibfield  {journal} {\bibinfo  {journal} {Phys. Rev. D}\ }\textbf {\bibinfo
  {volume} {101}},\ \bibinfo {pages} {105001} (\bibinfo {year} {2020})},\
  \Eprint {https://arxiv.org/abs/1911.06821} {arXiv:1911.06821 [hep-th]}
  \BibitemShut {NoStop}%
\bibitem [{\citenamefont {Choi}\ and\ \citenamefont
  {Akhoury}(2018)}]{sm-Choi:2017ylo}%
  \BibitemOpen
  \bibfield  {author} {\bibinfo {author} {\bibfnamefont {S.}~\bibnamefont
  {Choi}}\ and\ \bibinfo {author} {\bibfnamefont {R.}~\bibnamefont {Akhoury}},\
  }\bibfield  {title} {\bibinfo {title} {{BMS Supertranslation Symmetry Implies
  Faddeev-Kulish Amplitudes}},\ }\href
  {https://doi.org/10.1007/JHEP02(2018)171} {\bibfield  {journal} {\bibinfo
  {journal} {JHEP}\ }\textbf {\bibinfo {volume} {02}}\bibfield  {number}
  {\bibinfo  {number} { (2018)},\ \bibinfo {pages} {171}},\ }\Eprint
  {https://arxiv.org/abs/1712.04551} {arXiv:1712.04551 [hep-th]} \BibitemShut
  {NoStop}%
\bibitem [{\citenamefont {Cachazo}\ and\ \citenamefont
  {Strominger}(2014)}]{sm-CachazoStrominger:2014}%
  \BibitemOpen
  \bibfield  {author} {\bibinfo {author} {\bibfnamefont {F.}~\bibnamefont
  {Cachazo}}\ and\ \bibinfo {author} {\bibfnamefont {A.}~\bibnamefont
  {Strominger}},\ }\href@noop {} {\bibinfo {title} {{Evidence for a New Soft
  Graviton Theorem}}} (\bibinfo {year} {2014}),\ \Eprint
  {https://arxiv.org/abs/1404.4091} {arXiv:1404.4091 [hep-th]} \BibitemShut
  {NoStop}%
\bibitem [{\citenamefont {Sen}(2017)}]{sm-Sen:2017soft}%
  \BibitemOpen
  \bibfield  {author} {\bibinfo {author} {\bibfnamefont {A.}~\bibnamefont
  {Sen}},\ }\bibfield  {title} {\bibinfo {title} {{Soft Theorems in Superstring
  Theory}},\ }\href {https://doi.org/10.1007/JHEP06(2017)113} {\bibfield
  {journal} {\bibinfo  {journal} {JHEP}\ }\textbf {\bibinfo {volume}
  {06}}\bibfield  {number} {\bibinfo  {number} { (2017)},\ \bibinfo {pages}
  {113}},\ }\Eprint {https://arxiv.org/abs/1702.03934} {arXiv:1702.03934
  [hep-th]} \BibitemShut {NoStop}%
\bibitem [{\citenamefont {Sahoo}\ and\ \citenamefont
  {Sen}(2019)}]{sm-Sahoo:2018lxl}%
  \BibitemOpen
  \bibfield  {author} {\bibinfo {author} {\bibfnamefont {B.}~\bibnamefont
  {Sahoo}}\ and\ \bibinfo {author} {\bibfnamefont {A.}~\bibnamefont {Sen}},\
  }\bibfield  {title} {\bibinfo {title} {{Classical and Quantum Results on
  Logarithmic Terms in the Soft Theorem in Four Dimensions}},\ }\href
  {https://doi.org/10.1007/JHEP02(2019)086} {\bibfield  {journal} {\bibinfo
  {journal} {JHEP}\ }\textbf {\bibinfo {volume} {02}}\bibfield  {number}
  {\bibinfo  {number} { (2019)},\ \bibinfo {pages} {086}},\ }\Eprint
  {https://arxiv.org/abs/1808.03288} {arXiv:1808.03288 [hep-th]} \BibitemShut
  {NoStop}%
\bibitem [{\citenamefont {Ciafaloni}\ \emph {et~al.}(2016)\citenamefont
  {Ciafaloni}, \citenamefont {Colferai}, \citenamefont {Coradeschi},\ and\
  \citenamefont {Veneziano}}]{sm-Ciafaloni:2015unified}%
  \BibitemOpen
  \bibfield  {author} {\bibinfo {author} {\bibfnamefont {M.}~\bibnamefont
  {Ciafaloni}}, \bibinfo {author} {\bibfnamefont {D.}~\bibnamefont {Colferai}},
  \bibinfo {author} {\bibfnamefont {F.}~\bibnamefont {Coradeschi}},\ and\
  \bibinfo {author} {\bibfnamefont {G.}~\bibnamefont {Veneziano}},\ }\bibfield
  {title} {\bibinfo {title} {{Unified limiting form of graviton radiation at
  extreme energies}},\ }\href {https://doi.org/10.1103/PhysRevD.93.044052}
  {\bibfield  {journal} {\bibinfo  {journal} {Phys. Rev. D}\ }\textbf {\bibinfo
  {volume} {93}},\ \bibinfo {pages} {044052} (\bibinfo {year} {2016})},\
  \Eprint {https://arxiv.org/abs/1512.00281} {arXiv:1512.00281 [hep-th]}
  \BibitemShut {NoStop}%
\bibitem [{\citenamefont {Ciafaloni}\ \emph {et~al.}(2019)\citenamefont
  {Ciafaloni}, \citenamefont {Colferai},\ and\ \citenamefont
  {Veneziano}}]{sm-Ciafaloni:2019infrared}%
  \BibitemOpen
  \bibfield  {author} {\bibinfo {author} {\bibfnamefont {M.}~\bibnamefont
  {Ciafaloni}}, \bibinfo {author} {\bibfnamefont {D.}~\bibnamefont
  {Colferai}},\ and\ \bibinfo {author} {\bibfnamefont {G.}~\bibnamefont
  {Veneziano}},\ }\bibfield  {title} {\bibinfo {title} {{Infrared features of
  gravitational scattering and radiation in the eikonal approach}},\ }\href
  {https://doi.org/10.1103/PhysRevD.99.066008} {\bibfield  {journal} {\bibinfo
  {journal} {Phys. Rev. D}\ }\textbf {\bibinfo {volume} {99}},\ \bibinfo
  {pages} {066008} (\bibinfo {year} {2019})},\ \Eprint
  {https://arxiv.org/abs/1812.08137} {arXiv:1812.08137 [hep-th]} \BibitemShut
  {NoStop}%
\end{thebibliography}%
